# Supplementary material for: Adaptive Parallelism-Aware Qubit Routing for Ion Trap QCCD Architectures
Source: arXiv:2603.19969 source file (2026-03-20)
Supplement: Supplementary file 1 [file appendix.tex]

\appendix
\section*{APPENDIX}
\section*{Quantum algorithm behavior}
